# Supplementary material for: To Protect the LLM Agent Against the Prompt Injection Attack with Polymorphic Prompt
Source: arXiv:2506.05739 source file (2025-06-06)
Supplement: Supplementary file 1 [file appendix.tex]

\appendix

\footnotesize

\begin{longtable}{@{}p{14cm}r@{}}
\caption{List of Separators and Their Effectiveness.} \label{tab:comp_separators} \\

\toprule
\textbf{Separator} & \( \boldsymbol{P_i} \) \\
\midrule
\endfirsthead

\multicolumn{2}{c}%
{{\bfseries \tablename\ \thetable{} -- continued: Complete List of Separators and Their Effectiveness}} \\
\toprule
\textbf{Separator} & \( \boldsymbol{P_i} \) \\
\midrule
\endhead

\midrule \multicolumn{2}{r}{{Continued on next page}} \\
\endfoot

\bottomrule
\endlastfoot
        \texttt{['\#\#\#\#\# \{BEGIN\} \#\#\#\#\#', '\#\#\#\#\# \{END\} \#\#\#\#\#']} & 0.0\% \\
        \texttt{['\textasciitilde{}\textasciitilde{}\textasciitilde{}\textasciitilde{}\textasciitilde{}[START]\textasciitilde{}\textasciitilde{}\textasciitilde{}\textasciitilde{}\textasciitilde{}', '\textasciitilde{}\textasciitilde{}\textasciitilde{}\textasciitilde{}\textasciitilde{}[END]\textasciitilde{}\textasciitilde{}\textasciitilde{}\textasciitilde{}\textasciitilde{}']} & 0.0\% \\
        \texttt{['\textasciicircum{}\textasciicircum{}\textasciicircum{}\%\%\%\%\%\textasciicircum{}\textasciicircum{}\textasciicircum{}', '\textasciicircum{}\textasciicircum{}\textasciicircum{}\%\%\%\%\%\textasciicircum{}\textasciicircum{}\textasciicircum{}']} & 0.0\% \\
        \texttt{['!!!\#\#!!!\#\#!!!\#\#!!!', '!!!\#\#!!!\#\#!!!\#\#!!!']} & 0.0\% \\
        \texttt{['\#\#\#BEGIN\#\#\#', '\#\#\#END\#\#\#']} & 0.0\% \\
        \texttt{['===== BEGIN =====', '===== END =====']} & 0.0\% \\
        \texttt{['\#\#\#[BEGIN]\#\#\#', '\#\#\#[END]\#\#\#']} & 0.0\% \\
        \texttt{['\#\#\#@@@', '@@\#\#\#']} & 0.0\% \\
        \texttt{['*****START*****', '*****FINISH*****']} & 0.0\% \\
        \texttt{['\textasciitilde{}\textasciitilde{}\textasciitilde{}===\textasciitilde{}\textasciitilde{}\textasciitilde{}===\textasciitilde{}\textasciitilde{}\textasciitilde{}===\textasciitilde{}\textasciitilde{}\textasciitilde{}', '\textasciitilde{}\textasciitilde{}\textasciitilde{}===\textasciitilde{}\textasciitilde{}\textasciitilde{}===\textasciitilde{}\textasciitilde{}\textasciitilde{}===\textasciitilde{}\textasciitilde{}\textasciitilde{}']} & 0.0\% \\
        
\texttt{['\textasciitilde{}\textasciitilde{}\textasciitilde{}\textasciicircum{}\textasciicircum{}\textasciicircum{}\textasciitilde{}\textasciitilde{}\textasciitilde{}\textasciicircum{}\textasciicircum{}\textasciicircum{}\textasciitilde{}\textasciitilde{}\textasciitilde{}\textasciicircum{}\textasciicircum{}\textasciicircum{}\textasciitilde{}\textasciitilde{}\textasciitilde{}', '\textasciitilde{}\textasciitilde{}\textasciitilde{}\textasciicircum{}\textasciicircum{}\textasciicircum{}\textasciitilde{}\textasciitilde{}\textasciitilde{}\textasciicircum{}\textasciicircum{}\textasciicircum{}\textasciitilde{}\textasciitilde{}\textasciitilde{}\textasciicircum{}\textasciicircum{}\textasciicircum{}\textasciitilde{}\textasciitilde{}\textasciitilde{}']} & 0.0\% \\

\texttt{['\textasciicircum{}\textasciicircum{}\textasciicircum{}\#\#\#\textasciicircum{}\textasciicircum{}\textasciicircum{}\#\#\#\textasciicircum{}\textasciicircum{}\textasciicircum{}', '\textasciicircum{}\textasciicircum{}\textasciicircum{}\#\#\#\textasciicircum{}\textasciicircum{}\textasciicircum{}\#\#\#\textasciicircum{}\textasciicircum{}\textasciicircum{}']} & 0.0\% \\

\texttt{['///\#\#\#///\#\#\#///', '///\#\#\#///\#\#\#///']} & 0.0\% \\

\texttt{['///\textasciicircum{}\textasciicircum{}\textasciicircum{}///\textasciicircum{}\textasciicircum{}\textasciicircum{}///', '///\textasciicircum{}\textasciicircum{}\textasciicircum{}///\textasciicircum{}\textasciicircum{}\textasciicircum{}///']} & 0.0\% \\

\texttt{['///@@@///@@@///', '///@@@///@@@///']} & 0.0\% \\

\texttt{['>>>\{BEGIN\}>>>', '>>>\{END\}>>>']} & 0.0\% \\

\texttt{['*** START ***', '*** END ***']} & 0.0\% \\

\texttt{['****-{}-****-{}-****-{}-', '****-{}-****-{}-****-{}-']} & 0.0\% \\

\texttt{['\textasciitilde{}\textasciitilde{}\textasciitilde{}\textasciicircum{}\textasciicircum{}\textasciitilde{}\textasciitilde{}\textasciitilde{}\textasciicircum{}\textasciicircum{}\textasciitilde{}\textasciitilde{}\textasciitilde{}\textasciicircum{}\textasciicircum{}', '\textasciitilde{}\textasciitilde{}\textasciitilde{}\textasciicircum{}\textasciicircum{}\textasciitilde{}\textasciitilde{}\textasciitilde{}\textasciicircum{}\textasciicircum{}\textasciitilde{}\textasciitilde{}\textasciitilde{}\textasciicircum{}\textasciicircum{}']} & 0.0\% \\

\texttt{[``\#\#\#-{}-{}-\#\#\#-{}-{}-\#\#\#-{}-{}-\#\#\#'', ``\#\#\#-{}-{}-\#\#\#-{}-{}-\#\#\#-{}-{}-\#\#\#'']} & 0.0\% \\

\texttt{['\textasciicircum{}\textasciicircum{}\textasciicircum{}\$\$\$\textasciicircum{}\textasciicircum{}\textasciicircum{}\$\$\$\textasciicircum{}\textasciicircum{}\textasciicircum{}\$\$\$\textasciicircum{}', '\textasciicircum{}\textasciicircum{}\textasciicircum{}\$\$\$\textasciicircum{}\textasciicircum{}\textasciicircum{}\$\$\$\textasciicircum{}\textasciicircum{}\textasciicircum{}\$\$\$\textasciicircum{}']} & 0.0\% \\
\texttt{['\#\#\#***\#\#\#***\#\#\#***\#\#\#', '\#\#\#***\#\#\#***\#\#\#***\#\#\#']} & 0.0\% \\
\texttt{['===\#\#\#===\#\#\#===', '===\#\#\#===\#\#\#===']} & 0.0\% \\
\texttt{['\textasciitilde{}\textasciitilde{}\textasciitilde{}@@\textasciitilde{}\textasciitilde{}\textasciitilde{}@@\textasciitilde{}\textasciitilde{}\textasciitilde{}@@\textasciitilde{}\textasciitilde{}\textasciitilde{}@@', '\textasciitilde{}\textasciitilde{}\textasciitilde{}@@\textasciitilde{}\textasciitilde{}\textasciitilde{}@@\textasciitilde{}\textasciitilde{}\textasciitilde{}@@\textasciitilde{}\textasciitilde{}\textasciitilde{}@@']} & 0.0\% \\
\texttt{['\textasciitilde{}\textasciitilde{}\textasciitilde{}///\textasciitilde{}\textasciitilde{}\textasciitilde{}///\textasciitilde{}\textasciitilde{}\textasciitilde{}///\textasciitilde{}\textasciitilde{}\textasciitilde{}', '\textasciitilde{}\textasciitilde{}\textasciitilde{}///\textasciitilde{}\textasciitilde{}\textasciitilde{}///\textasciitilde{}\textasciitilde{}\textasciitilde{}///\textasciitilde{}\textasciitilde{}\textasciitilde{}']} & 0.0\% \\

\texttt{['\textasciicircum{}\textasciicircum{}\textasciicircum{}***\textasciicircum{}\textasciicircum{}\textasciicircum{}***\textasciicircum{}\textasciicircum{}\textasciicircum{}***\textasciicircum{}', '\textasciicircum{}\textasciicircum{}\textasciicircum{}***\textasciicircum{}\textasciicircum{}\textasciicircum{}***\textasciicircum{}\textasciicircum{}\textasciicircum{}***\textasciicircum{}']} & 0.0\% \\
% \texttt{['===\#\#\#===\#\#\#===', '===\#\#\#===\#\#\#===']} & 0.0\% \\
% \texttt{['\textasciicircum{}\textasciicircum{}\textasciicircum{}\#\#\#\textasciicircum{}\textasciicircum{}\textasciicircum{}\#\#\#\textasciicircum{}\textasciicircum{}\textasciicircum{}', '\textasciicircum{}\textasciicircum{}\textasciicircum{}\#\#\#\textasciicircum{}\textasciicircum{}\textasciicircum{}\#\#\#\textasciicircum{}\textasciicircum{}\textasciicircum{}']} & 0.0\% \\
% \texttt{['***\&\&\&***\&\&\&***', '***\&\&\&***\&\&\&***']} & 0.0\% \\
\texttt{['\textasciitilde{}\textasciitilde{}\textasciitilde{}***\textasciitilde{}\textasciitilde{}\textasciitilde{}***\textasciitilde{}\textasciitilde{}\textasciitilde{}', '\textasciitilde{}\textasciitilde{}\textasciitilde{}***\textasciitilde{}\textasciitilde{}\textasciitilde{}***\textasciitilde{}\textasciitilde{}\textasciitilde{}']} & 0.0\% \\

% \texttt{['///@@@///@@@///', '///@@@///@@@///']} & 0.0\% \\
\texttt{['===@@@===@@@===', '===@@@===@@@===']} & 0.0\% \\
\texttt{['\textasciitilde{}\textasciitilde{}\textasciitilde{}\textasciitilde{}\textasciitilde{}\{START\}\textasciitilde{}\textasciitilde{}\textasciitilde{}\textasciitilde{}\textasciitilde{}', '\textasciitilde{}\textasciitilde{}\textasciitilde{}\textasciitilde{}\textasciitilde{}\{END\}\textasciitilde{}\textasciitilde{}\textasciitilde{}\textasciitilde{}\textasciitilde{}']} & 0.0\% \\
\texttt{['>{}>{}>{}>{}>[START]>{}>{}>{}>{}>', '>{}>{}>{}>{}>[END]>{}>{}>{}>{}>']} & 0.0\% \\
\texttt{['\#\#\#\$\$\$\%\%\% [BEGIN] \%\%\%\$\$\$\#\#\#', '\#\#\#\$\$\$\%\%\% [END] \%\%\%\$\$\$\#\#\#']} & 0.0\% \\

\texttt{['\textasciicircum{}\textasciicircum{}\textasciicircum{}!!\textasciicircum{}\textasciicircum{}\textasciicircum{}!!\textasciicircum{}\textasciicircum{}\textasciicircum{}!!\textasciicircum{}\textasciicircum{}\textasciicircum{}!!', '\textasciicircum{}\textasciicircum{}\textasciicircum{}!!\textasciicircum{}\textasciicircum{}\textasciicircum{}!!\textasciicircum{}\textasciicircum{}\textasciicircum{}!!\textasciicircum{}\textasciicircum{}\textasciicircum{}!!']} & 0.0\% \\
\texttt{['\#\#\#---[START]---\#\#\#', '\#\#\#---[END]---\#\#\#']} & 0.0\% \\
\texttt{['\textasciitilde{}\textasciitilde{}\textasciitilde{}@@\textasciitilde{}\textasciitilde{}\textasciitilde{}@@\textasciitilde{}\textasciitilde{}\textasciitilde{}@@\textasciitilde{}\textasciitilde{}\textasciitilde{}', '\textasciitilde{}\textasciitilde{}\textasciitilde{}@@\textasciitilde{}\textasciitilde{}\textasciitilde{}@@\textasciitilde{}\textasciitilde{}\textasciitilde{}@@\textasciitilde{}\textasciitilde{}\textasciitilde{}']} & 5.0\% \\
\texttt{['>{}>{}>START>{}>{}>', '>{}>{}>FINISH>{}>{}>']} & 5.0\% \\
\texttt{['\textasciitilde{}\textasciitilde{}\textasciitilde{}\textasciitilde{}\textasciitilde{}(BEGIN)\textasciitilde{}\textasciitilde{}\textasciitilde{}\textasciitilde{}\textasciitilde{}', '\textasciitilde{}\textasciitilde{}\textasciitilde{}\textasciitilde{}\textasciitilde{}(FINISH)\textasciitilde{}\textasciitilde{}\textasciitilde{}\textasciitilde{}\textasciitilde{}']} & 5.0\% \\

\texttt{['-{}-{}-{}-{}-BEGIN-{}-{}-{}-{}-', '-{}-{}-{}-{}-END-{}-{}-{}-{}-']} & 5.0\% \\
\texttt{['===++===++===++===++', '===++===++===++===++']} & 5.0\% \\
\texttt{['\textasciicircum{}\textasciicircum{}\textasciicircum{}@@@\textasciicircum{}\textasciicircum{}\textasciicircum{}@@@\textasciicircum{}\textasciicircum{}\textasciicircum{}@@@', '\textasciicircum{}\textasciicircum{}\textasciicircum{}@@@\textasciicircum{}\textasciicircum{}\textasciicircum{}@@@\textasciicircum{}\textasciicircum{}\textasciicircum{}@@@']} & 5.0\% \\
\texttt{['///-{}-{}-\{BEGIN\}-{}-{}-///', '///-{}-{}-\{END\}-{}-{}-///']} & 5.0\% \\
\texttt{['***START***', '***END***']} & 5.0\% \\

\texttt{['*****[START]*****', '*****[STOP]*****']} & 5.0\% \\
% \texttt{['\#\#\#BEGIN\#\#\#', '\#\#\#END\#\#\#']} & 5.0\% \\
\texttt{['\textasciitilde{} BEGIN \textasciitilde{}', '\textasciitilde{} END \textasciitilde{}']} & 5.0\% \\
\texttt{['>{}>==>{}>==>{}>==>{}>==', '>{}>==>{}>==>{}>==>{}>==']} & 5.0\% \\
\texttt{['\#\#\#@@\#\#\#@@\#\#\#@@\#\#\#@@', '\#\#\#@@\#\#\#@@\#\#\#@@\#\#\#@@']} & 5.0\% \\

% \texttt{['===\#\#\#===\#\#\#===', '===\#\#\#===\#\#\#===']} & 5.0\% \\
% \texttt{['===\&\&\&===\&\&\&===', '===\&\&\&===\&\&\&===']} & 5.0\% \\
% \texttt{['|||START|||', '|||END|||']} & 5.0\% \\
\texttt{['***BEGIN***', '***END***']} & 5.0\% \\
% \texttt{['*** START ***', '*** END ***']} & 5.0\% \\

\texttt{['>{}>{}> START >{}>{}>', '<{}<{}< END <{}<{}<']} & 5.0\% \\
% \texttt{['\#\#\#[BEGIN]\#\#\#', '\#\#\#[END]\#\#\#']} & 5.0\% \\
\texttt{['\textasciitilde{}\textasciitilde{}\textasciitilde{}+++\textasciitilde{}\textasciitilde{}\textasciitilde{}+++\textasciitilde{}\textasciitilde{}\textasciitilde{}+++\textasciitilde{}\textasciitilde{}\textasciitilde{}', '\textasciitilde{}\textasciitilde{}\textasciitilde{}+++\textasciitilde{}\textasciitilde{}\textasciitilde{}+++\textasciitilde{}\textasciitilde{}\textasciitilde{}+++\textasciitilde{}\textasciitilde{}\textasciitilde{}']} & 5.0\% \\
% \texttt{['\textasciitilde{}\textasciitilde{}\textasciitilde{}===\textasciitilde{}\textasciitilde{}\textasciitilde{}===\textasciitilde{}\textasciitilde{}\textasciitilde{}===\textasciitilde{}\textasciitilde{}\textasciitilde{}', '\textasciitilde{}\textasciitilde{}\textasciitilde{}===\textasciitilde{}\textasciitilde{}\textasciitilde{}===\textasciitilde{}\textasciitilde{}\textasciitilde{}===\textasciitilde{}\textasciitilde{}\textasciitilde{}']} & 5.0\% \\
\texttt{['\%\%\%-{}-{}-\%\%\%-{}-{}-\%\%\%-{}-{}-\%\%\%', '\%\%\%-{}-{}-\%\%\%-{}-{}-\%\%\%-{}-{}-\%\%\%']} & 5.0\% \\

% \texttt{['\textasciitilde{}\textasciitilde{}\textasciitilde{}***\textasciitilde{}\textasciitilde{}\textasciitilde{}***\textasciitilde{}\textasciitilde{}\textasciitilde{}', '\textasciitilde{}\textasciitilde{}\textasciitilde{}***\textasciitilde{}\textasciitilde{}\textasciitilde{}***\textasciitilde{}\textasciitilde{}\textasciitilde{}']} & 5.0\% \\
\texttt{['\#\#\#\%\%\%\#\#\#\%\%\%\#\#\#', '\#\#\#\%\%\%\#\#\#\%\%\%\#\#\#']} & 5.0\% \\
\texttt{['\#\#\#==\#\#\#==\#\#\#==\#\#\#==', '\#\#\#==\#\#\#==\#\#\#==\#\#\#==']} & 5.0\% \\
\texttt{['>{}>{}>===>{}>{}>===>{}>{}>===>{}>{}>', '>{}>{}>===>{}>{}>===>{}>{}>===>{}>{}>']} & 5.0\% \\
\texttt{['\#\#\#**\#\#\#**\#\#\#**\#\#\#**', '\#\#\#**\#\#\#**\#\#\#**\#\#\#**']} & 5.0\% \\

\texttt{['===@@===@@===@@===@@', '===@@===@@===@@===@@']} & 5.0\% \\
\texttt{['\#\#\#-{}-{}-\#\#\#-{}-{}-\#\#\#-{}-{}-\#\#\#', '\#\#\#-{}-{}-\#\#\#-{}-{}-\#\#\#-{}-{}-\#\#\#']} & 5.0\% \\
\texttt{['+++=\!=+++=\!=+++=\!=+++', '+++=\!=+++=\!=+++=\!=+++']} & 5.0\% \\
\texttt{['===\%\%\%===\%\%\%===', '===\%\%\%===\%\%\%===']} & 5.0\% \\
\texttt{['\textasciitilde{}\textasciitilde{}\textasciitilde{}@@@\textasciitilde{}\textasciitilde{}\textasciitilde{}@@@\textasciitilde{}\textasciitilde{}\textasciitilde{}', '\textasciitilde{}\textasciitilde{}\textasciitilde{}@@@\textasciitilde{}\textasciitilde{}\textasciitilde{}@@@\textasciitilde{}\textasciitilde{}\textasciitilde{}']} & 5.0\% \\

\texttt{['***\&\&\&***\&\&\&***', '***\&\&\&***\&\&\&***']} & 5.0\% \\
\texttt{['///\$\$\$///\$\$\$///', '///\$\$\$///\$\$\$///']} & 5.0\% \\
\texttt{['\textasciicircum{}\textasciicircum{}\textasciicircum{}\%\%\%\textasciicircum{}\textasciicircum{}\textasciicircum{}\%\%\%\textasciicircum{}\textasciicircum{}\textasciicircum{}', '\textasciicircum{}\textasciicircum{}\textasciicircum{}\%\%\%\textasciicircum{}\textasciicircum{}\textasciicircum{}\%\%\%\textasciicircum{}\textasciicircum{}\textasciicircum{}']} & 5.0\% \\
\texttt{['+++\#\#\#+++\#\#\#+++', '+++\#\#\#+++\#\#\#+++']} & 5.0\% \\
\texttt{['\#\#\#==\#\#\#==\#\#\#', '\#\#\#==\#\#\#==\#\#\#']} & 5.0\% \\

\texttt{['///\textasciicircum{}\textasciicircum{}\textasciicircum{}///\textasciicircum{}\textasciicircum{}\textasciicircum{}///\textasciicircum{}\textasciicircum{}\textasciicircum{}', '///\textasciicircum{}\textasciicircum{}\textasciicircum{}///\textasciicircum{}\textasciicircum{}\textasciicircum{}///\textasciicircum{}\textasciicircum{}\textasciicircum{}']} & 5.0\% \\
\texttt{['***@@@***@@@***', '***@@@***@@@***']} & 5.0\% \\
\texttt{['<{}<{}<[START]>{}>{}>', '<{}<{}<[END]>{}>{}>']} & 5.0\% \\
\texttt{['\#\#\#\{BEGIN\}\#\#\#', '\#\#\#\{END\}\#\#\#']} & 5.0\% \\
\texttt{['*****[START]*****', '*****[END]*****']} & 5.0\% \\

\texttt{['\#\#\#\#\#(START)\#\#\#\#\#', '\#\#\#\#\#(END)\#\#\#\#\#']} & 5.0\% \\
\texttt{['\textasciitilde{}\textasciitilde{}\textasciitilde{}\$\$\textasciitilde{}\textasciitilde{}\textasciitilde{}\$\$\textasciitilde{}\textasciitilde{}\textasciitilde{}\$\$\textasciitilde{}\textasciitilde{}\textasciitilde{}\$\$', '\textasciitilde{}\textasciitilde{}\textasciitilde{}\$\$\textasciitilde{}\textasciitilde{}\textasciitilde{}\$\$\textasciitilde{}\textasciitilde{}\textasciitilde{}\$\$\textasciitilde{}\textasciitilde{}\textasciitilde{}\$\$']} & 5.0\% \\
\texttt{['\#\#\#\#\#\#\#\#START\#\#\#\#\#\#\#\#', '\#\#\#\#\#\#\#\#END\#\#\#\#\#\#\#\#']} & 5.0\% \\
\texttt{['\#\#\#\#\#\#\#\#\#\#[BEGIN]\#\#\#\#\#\#\#\#\#\#', '\#\#\#\#\#\#\#\#\#\#[END]\#\#\#\#\#\#\#\#\#\#']} & 5.0\% \\

\end{longtable}
